# Supplementary material for: Stockmayer supracolloidal magnetic polymers under the influence of an applied magnetic field and a shear flow
Source: arXiv:2306.03005 source file (2023-06-05)
Supplement: Supplementary file 1 [file suplementary.tex]

\documentclass[twoside,twocolumn,9pt]{article}
\usepackage{extsizes}
\usepackage[singlespacing]{setspace}
\usepackage[super,sort&compress,comma]{natbib} 
\usepackage[version=3]{mhchem}
\usepackage[left=1.5cm, right=1.5cm, top=1.785cm, bottom=2.0cm,]{geometry}
\usepackage{balance}
\usepackage{widetext}
\usepackage{times,mathptmx}
\usepackage{sectsty}
\usepackage{graphicx} 
\usepackage{lastpage}
\usepackage[format=plain,justification=raggedright,singlelinecheck=false,font={stretch=1.125,small,sf},labelfont=bf,labelsep=space]{caption}
\usepackage{float}
\usepackage{fancyhdr}
\usepackage{fnpos}
\usepackage[english]{babel}
\usepackage{array}
\usepackage{droidsans}
\usepackage{dblfloatfix}
\usepackage{charter}
\usepackage[T1]{fontenc}
\usepackage[usenames,dvipsnames]{xcolor}
\usepackage{setspace}
\usepackage[compact]{titlesec}
\usepackage{subfigure}
%%%Please don't disable any packages in the preamble, as this may cause the template to display incorrectly.%%%

% \usepackage{epstopdf}%This line makes .eps figures into .pdf - please comment out if not required.

\definecolor{cream}{RGB}{222,217,201}

\begin{document}
\showthe\textwidth
\showthe\columnwidth
\pagestyle{fancy}
\thispagestyle{plain}
\fancypagestyle{plain}{

%%%HEADER%%%
\fancyhead[C]{\includegraphics[width=18.5cm]{head_foot/header_bar}}
\fancyhead[L]{\hspace{0cm}\vspace{1.5cm}\includegraphics[height=30pt]{head_foot/journal_name}}
\fancyhead[R]{\hspace{0cm}\vspace{1.7cm}\includegraphics[height=55pt]{head_foot/RSC_LOGO_CMYK}}
\renewcommand{\headrulewidth}{0pt}
}
%%%END OF HEADER%%%

%%%PAGE SETUP - Please do not change any commands within this section%%%
\makeFNbottom
\makeatletter
\renewcommand\LARGE{\@setfontsize\LARGE{15pt}{17}}
\renewcommand\Large{\@setfontsize\Large{12pt}{14}}
\renewcommand\large{\@setfontsize\large{10pt}{12}}
\renewcommand\footnotesize{\@setfontsize\footnotesize{7pt}{10}}
\makeatother

\renewcommand{\thefootnote}{\fnsymbol{footnote}}
\renewcommand\footnoterule{\vspace*{1pt}% 
\color{cream}\hrule width 3.5in height 0.4pt \color{black}\vspace*{5pt}} 
\setcounter{secnumdepth}{5}

\makeatletter 
\renewcommand\@biblabel[1]{#1}            
\renewcommand\@makefntext[1]% 
{\noindent\makebox[0pt][r]{\@thefnmark\,}#1}
\makeatother 
\renewcommand{\figurename}{\small{Fig.}~}
\sectionfont{\sffamily\Large}
\subsectionfont{\normalsize}
\subsubsectionfont{\bf}
\setstretch{1.125} %In particular, please do not alter this line.
\setlength{\skip\footins}{0.8cm}
\setlength{\footnotesep}{0.25cm}
\setlength{\jot}{10pt}
\titlespacing*{\section}{0pt}{4pt}{4pt}
\titlespacing*{\subsection}{0pt}{15pt}{1pt}
%%%END OF PAGE SETUP%%%

%%%FOOTER%%%
\fancyfoot{}
\fancyfoot[LO,RE]{\vspace{-7.1pt}\includegraphics[height=9pt]{head_foot/LF}}
\fancyfoot[CO]{\vspace{-7.1pt}\hspace{13.2cm}\includegraphics{head_foot/RF}}
\fancyfoot[CE]{\vspace{-7.2pt}\hspace{-14.2cm}\includegraphics{head_foot/RF}}
\fancyfoot[RO]{\footnotesize{\sffamily{1--\pageref{LastPage} ~\textbar  \hspace{2pt}\thepage}}}
\fancyfoot[LE]{\footnotesize{\sffamily{\thepage~\textbar\hspace{3.45cm} 1--\pageref{LastPage}}}}
\fancyhead{}
\renewcommand{\headrulewidth}{0pt} 
\renewcommand{\footrulewidth}{0pt}
\setlength{\arrayrulewidth}{1pt}
\setlength{\columnsep}{6.5mm}
\setlength\bibsep{1pt}
%%%END OF FOOTER%%%

%%%FIGURE SETUP - please do not change any commands within this section%%%
\makeatletter 
\newlength{\figrulesep} 
\setlength{\figrulesep}{0.5\textfloatsep} 

\newcommand{\topfigrule}{\vspace*{-1pt}% 
\noindent{\color{cream}\rule[-\figrulesep]{\columnwidth}{1.5pt}} }

\newcommand{\botfigrule}{\vspace*{-2pt}% 
\noindent{\color{cream}\rule[\figrulesep]{\columnwidth}{1.5pt}} }

\newcommand{\dblfigrule}{\vspace*{-1pt}% 
\noindent{\color{cream}\rule[-\figrulesep]{\textwidth}{1.5pt}} }

\makeatother
%%%END OF FIGURE SETUP%%%

%%%TITLE, AUTHORS AND ABSTRACT%%%
\twocolumn[
  \begin{@twocolumnfalse}
\vspace{3cm}
\sffamily
\begin{tabular}{m{4.5cm} p{13.5cm} }

\includegraphics{head_foot/DOI} & \noindent\LARGE{\textbf{Supplementary for Stockmayer supracolloidal magnetic polymers under the influence of an applied magnetic field and a shear flow}} \\%Article title goes here instead of the text "This is the title"
\vspace{0.3cm} & \vspace{0.3cm} \\

 & \noindent\large{Ivan S. Novikau,\textit{$^{a}$}Vladimir S. Novak,\textit{$^{b}$}Ekaterina V. Novak,\textit{$^{b}$} and Sofia S. Kantorovich$^{\ast}$\textit{$^{a,c}$}} \\%Author names go here instead of "Full name", etc.

\includegraphics{head_foot/dates} & 
\end{tabular}

 \end{@twocolumnfalse} \vspace{0.6cm}

]%%%END OF TITLE, AUTHORS AND ABSTRACT%%%

%%%FONT SETUP - please do not change any commands within this section
\renewcommand*\rmdefault{bch}\normalfont\upshape
\rmfamily
\section*{}
\vspace{-1cm}

%%%FOOTNOTES%%%

\footnotetext{\textit{$^{a}$~University of Vienna, Vienna, Austria.; Tel:+43-1-4277-73277; E-mail: deniz.mostarac@univie.ac.at}}
\footnotetext{\textit{$^{b}$~Ural Federal University, Ekaterinburg, Russia. }}
\footnotetext{\textit{$^{c}$~Research Platform ``Mathematics-Magnetism-Materials, University of Vienna, Oskar-Morgenstern-Platz 1, Vienna, Austria. }}
%Please use \dag to cite the ESI in the main text of the article.
%If you article does not have ESI please remove the the \dag symbol from the title and the footnotetext below.

%additional addresses can be cited as above using the lower-case letters, c, d, e... If all authors are from the same address, no letter is required

%%%END OF FOOTNOTES%%%
%%%MAIN TEXT%%%%

In this part of the manuscript we provide extra plots for magnetisation behaviour to support our main conclusions. 

In Fig. \ref{fig:sup-mag-a} we plot the dependence of $\mu^{\ast}$ for chain, ring, and Y-like clusters for three field orientations. This figure is similar to Fig. 7 of the main article. It can be clearly seen that independently of the shear rate and field strength only linear regime is observed for the clusters formed by linear and ring-like SSMPs (first two rows). Mild nonlinear effects can be found in the lowest row, where $\mu^{\ast}$ for clusters made of Y-like SSMPs is plotted, in particular if $\dot{\gamma}$ is high.

\begin{figure*}[h!]
    \centering
    \includegraphics[width=0.55\linewidth]{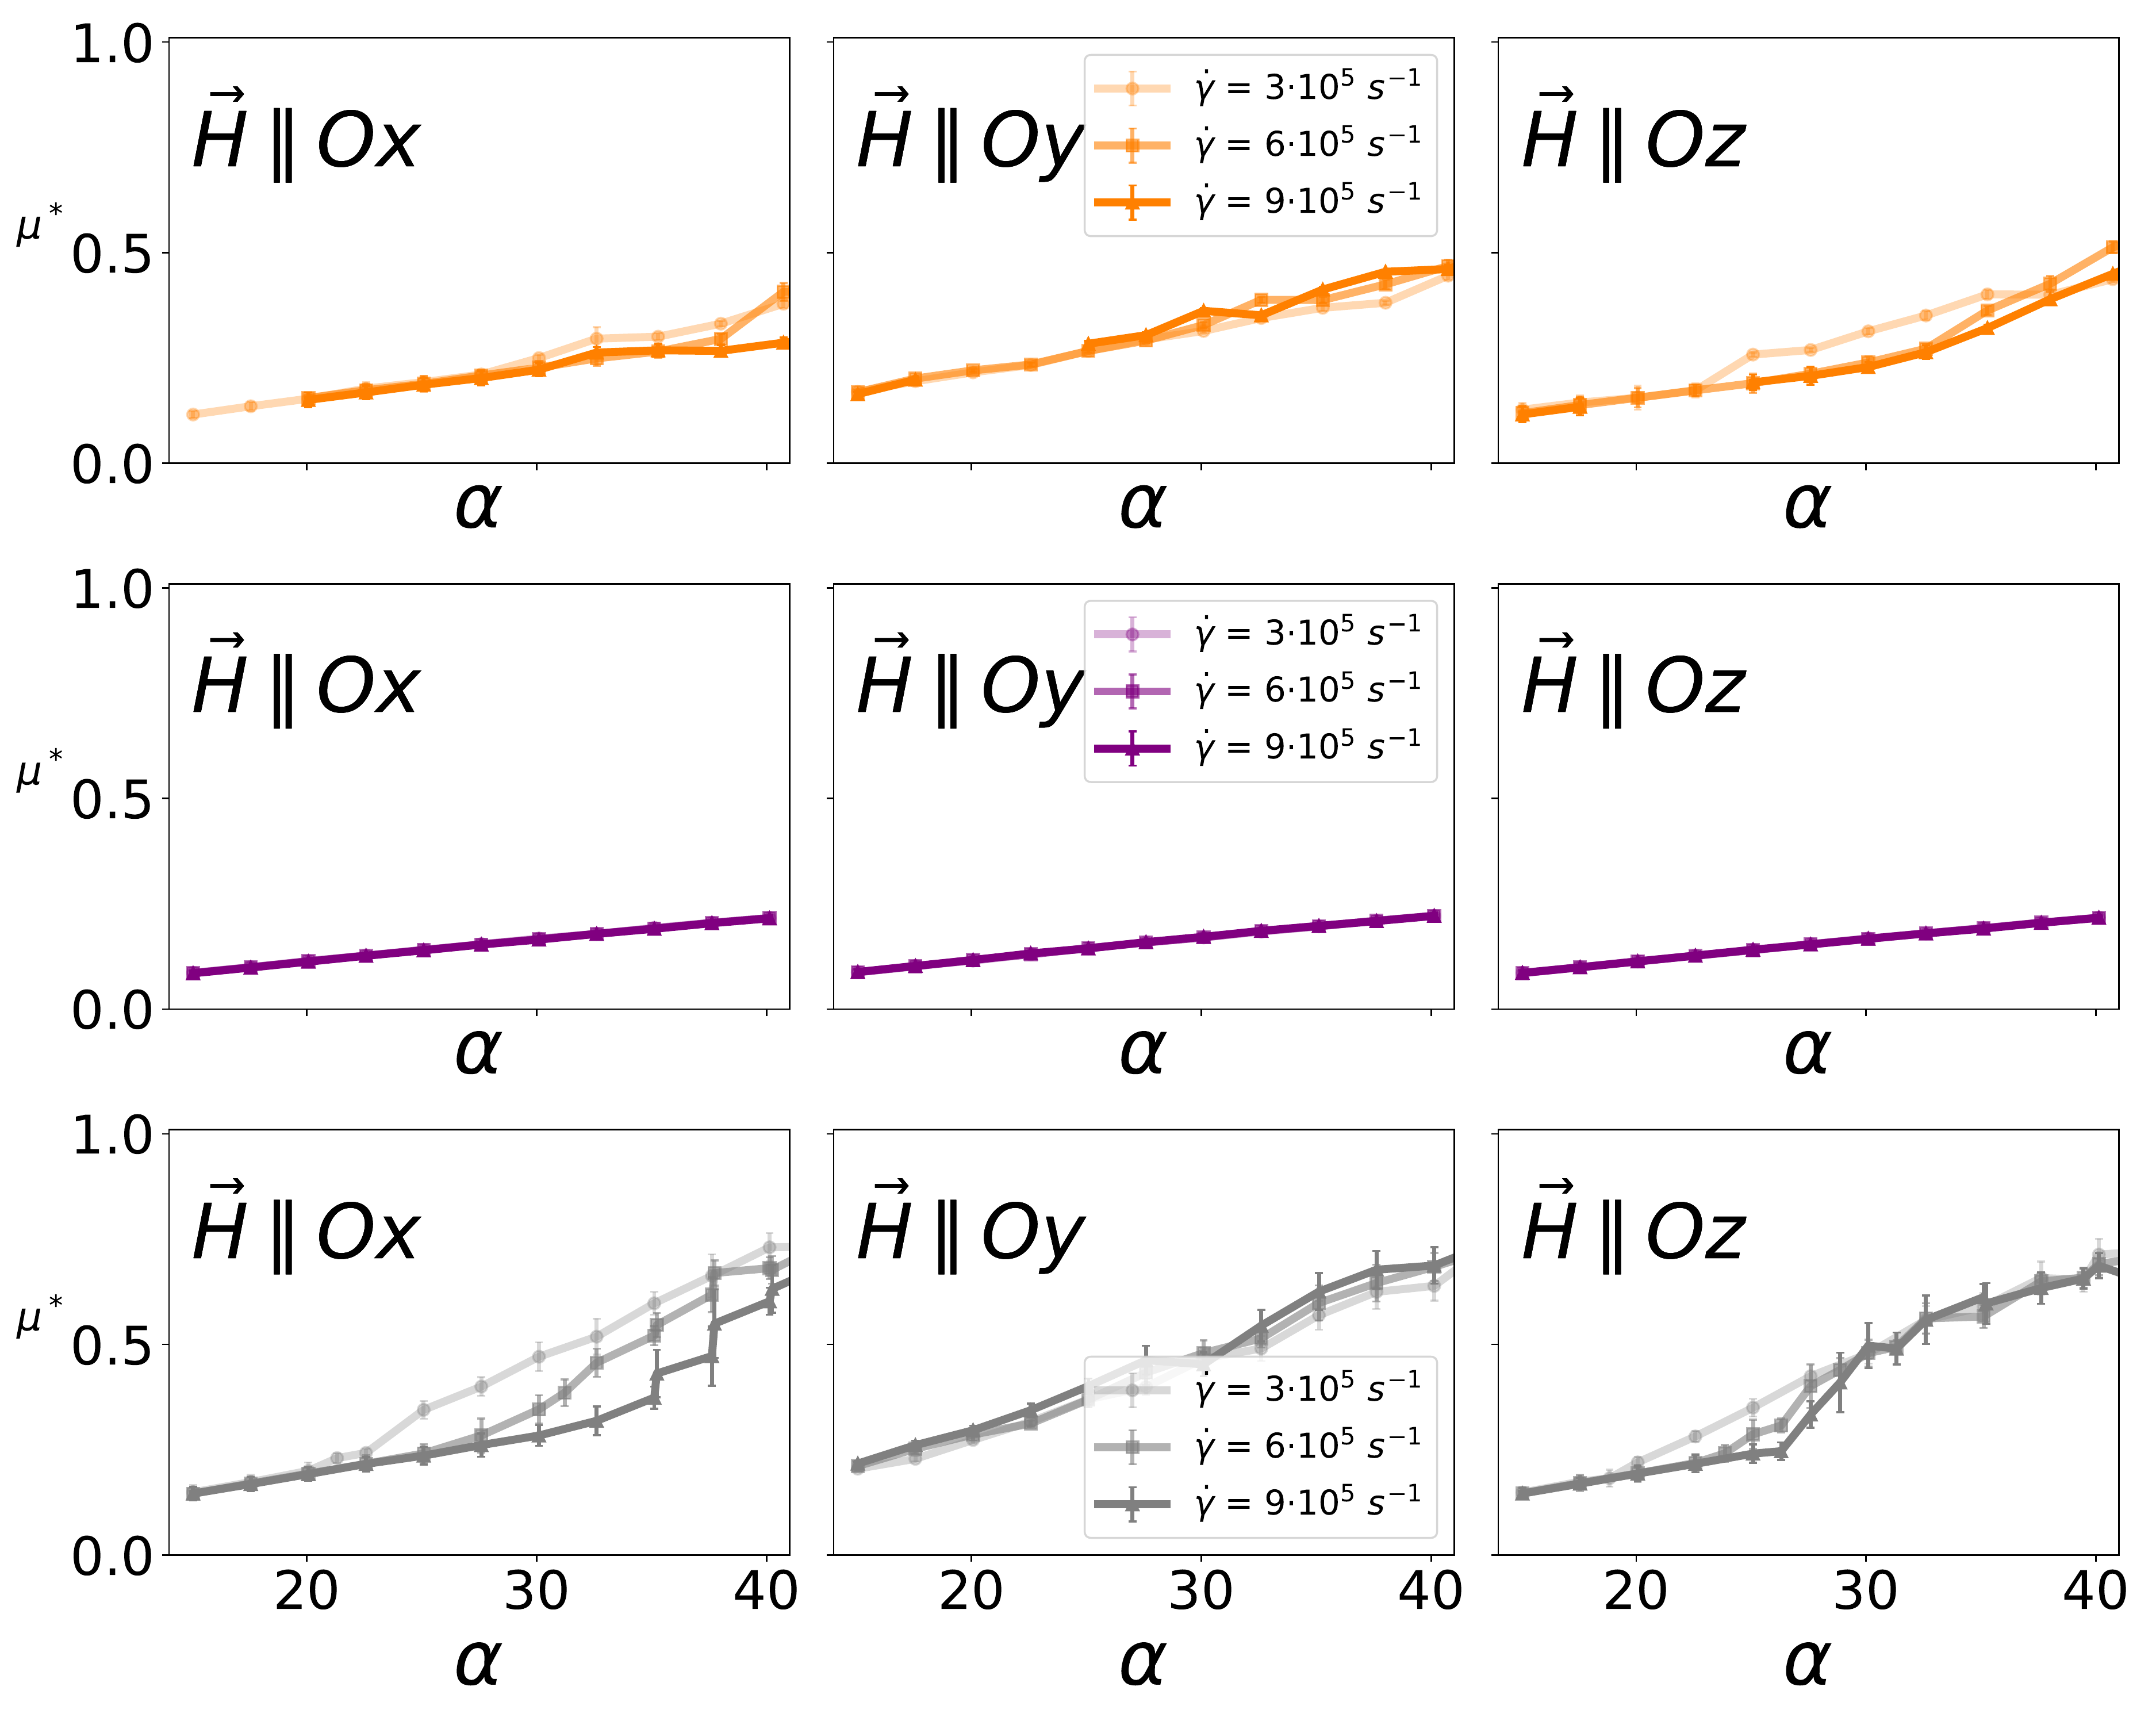}
    \caption{Magnetisation $\mu^{\ast}$ for chain, ring, and Y-like clusters for the field aligned with Ox, Oy, Oz. The brightness of the curves corresponds to the value of the shear rate -- the darker the curve, the higher the value of $\dot{\gamma}$. Exact $\dot{\gamma}$ values and orientation of the applied field are provided in the insets.}\label{fig:sup-mag-a}
\end{figure*}

In Figs. 2--4 we collected magnetisation dynamics for chain, ring, and Y-like clusters for three field orientations and selected field intensities, similarly to Fig. 9 of the main manuscript. It is easy to see that as mentioned in the main text the same three regimes for the magnetisation dynamics can be observed for all but one cluster types: the clusters made of rings are not responding to an applied field investigated in this study. As expected, the least oscillations (after clusters made of X-like SSMPs) are found in Fig. 2 for the case of SSMP Y topology.

\begin{figure*}[h]
\begin{minipage}[h]{\linewidth}
\center{\includegraphics[width=0.7\linewidth]{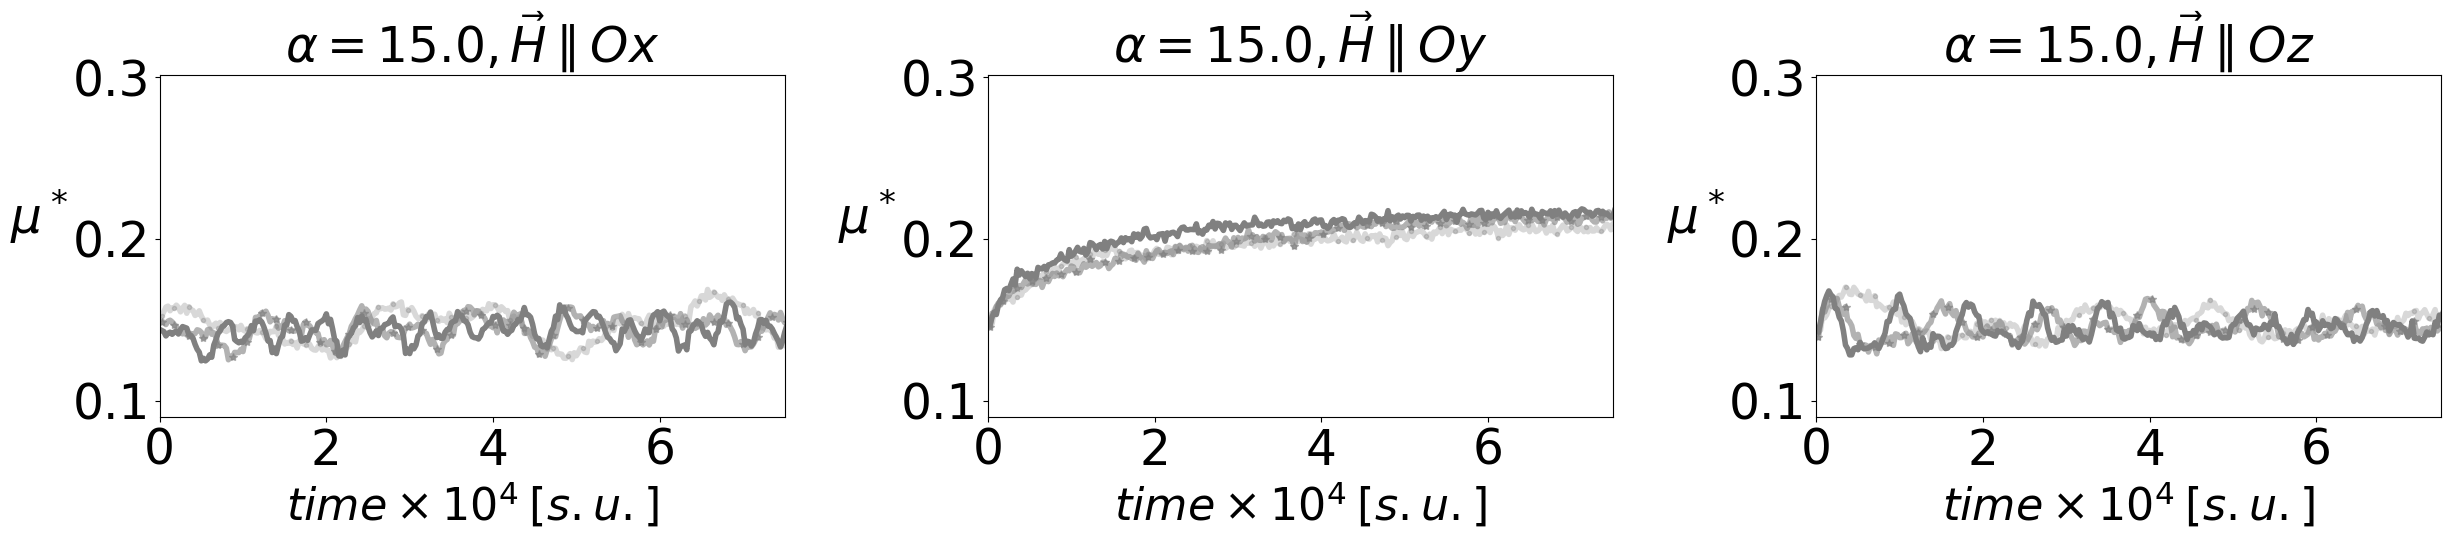} }
\end{minipage}
\vfill
\begin{minipage}[h]{\linewidth}
\center{\includegraphics[width=0.7\linewidth]{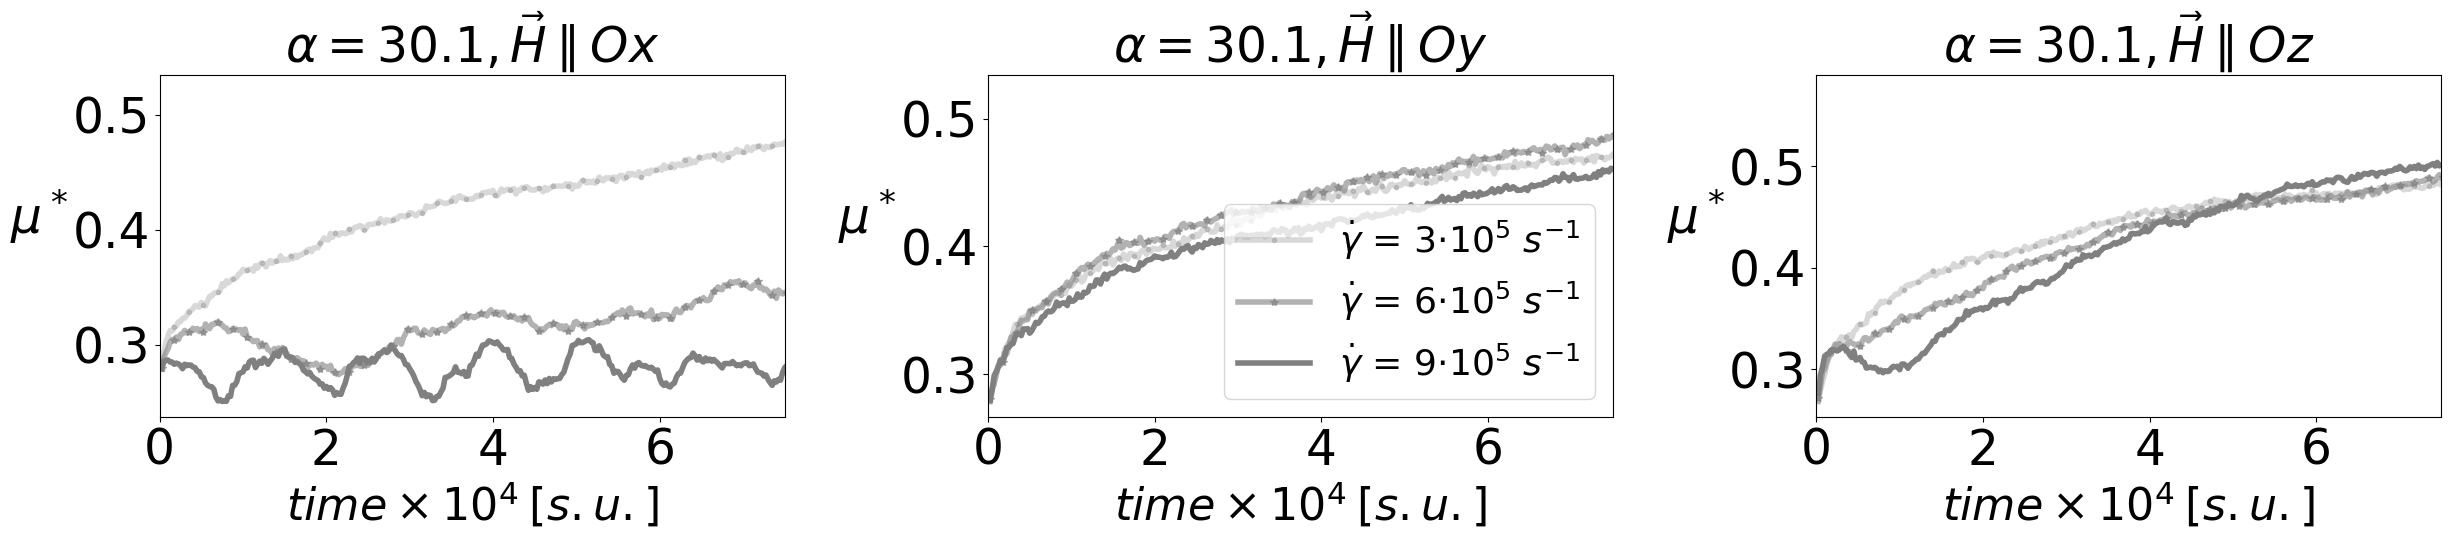} }
\end{minipage}
\vfill
\begin{minipage}[h]{\linewidth}
\center{\includegraphics[width=0.7\linewidth]{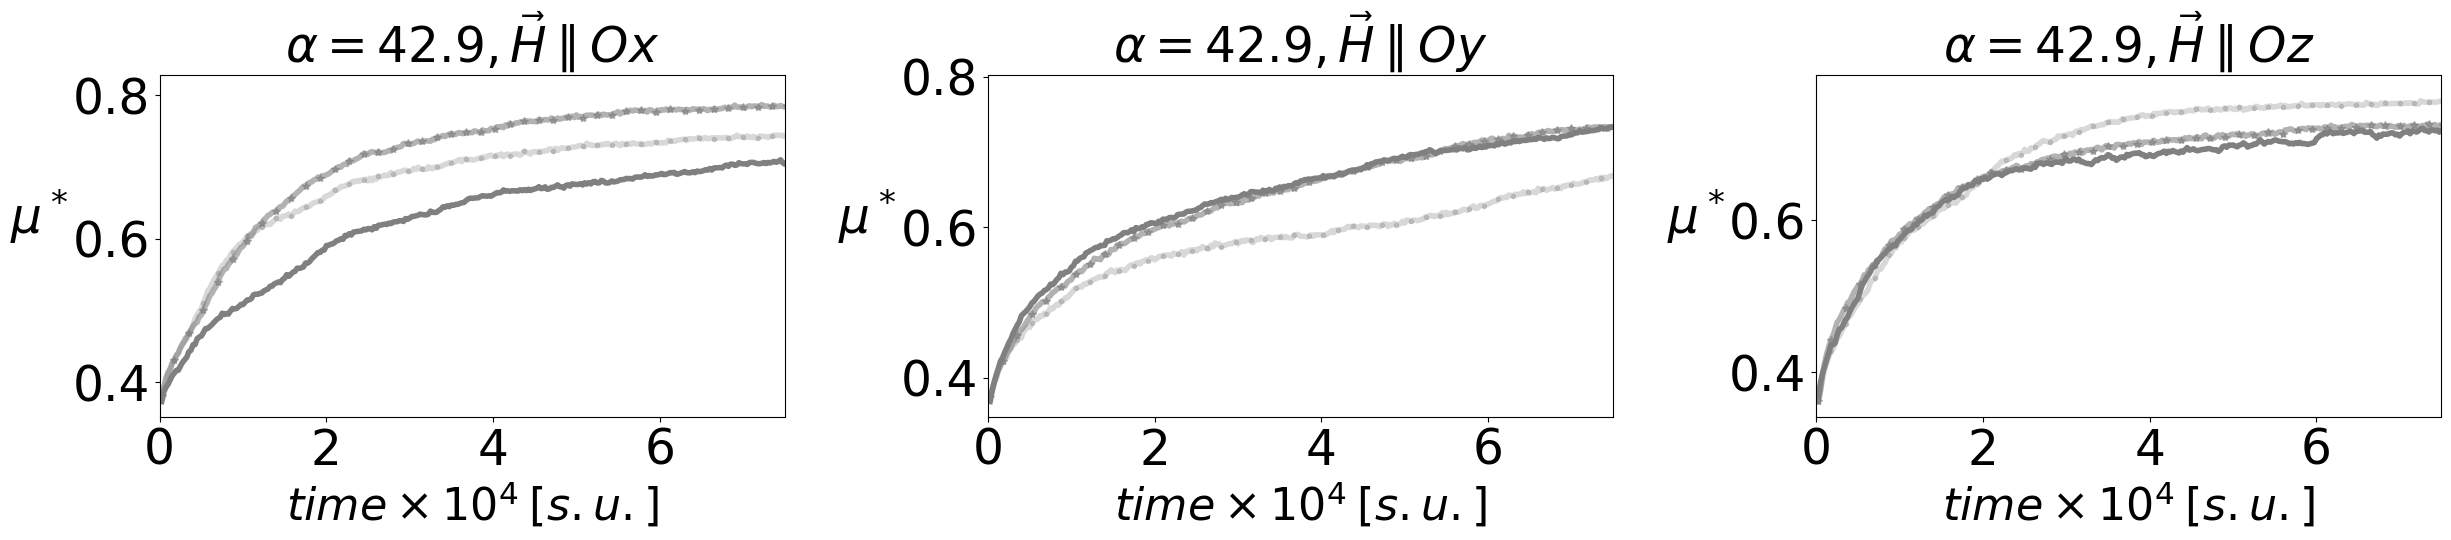} }
\end{minipage}
\caption{Dynamics of the magnetisation $\mu^{\ast}$ for a Y topology of the SSMPs. Columns correspond to a given orientation of the applied field. The brightness of the curves corresponds to the value of the shear rate -- the darker the curve, the higher the value of $\dot{\gamma}$. Exact $\dot{\gamma}$ values are provided in the inset of central. Field is fixed within each row. Values of $\alpha$ are provided above the plots.}
\end{figure*}

\begin{figure*}[h]
\begin{minipage}[h]{\linewidth}
\center{\includegraphics[width=0.7\linewidth]{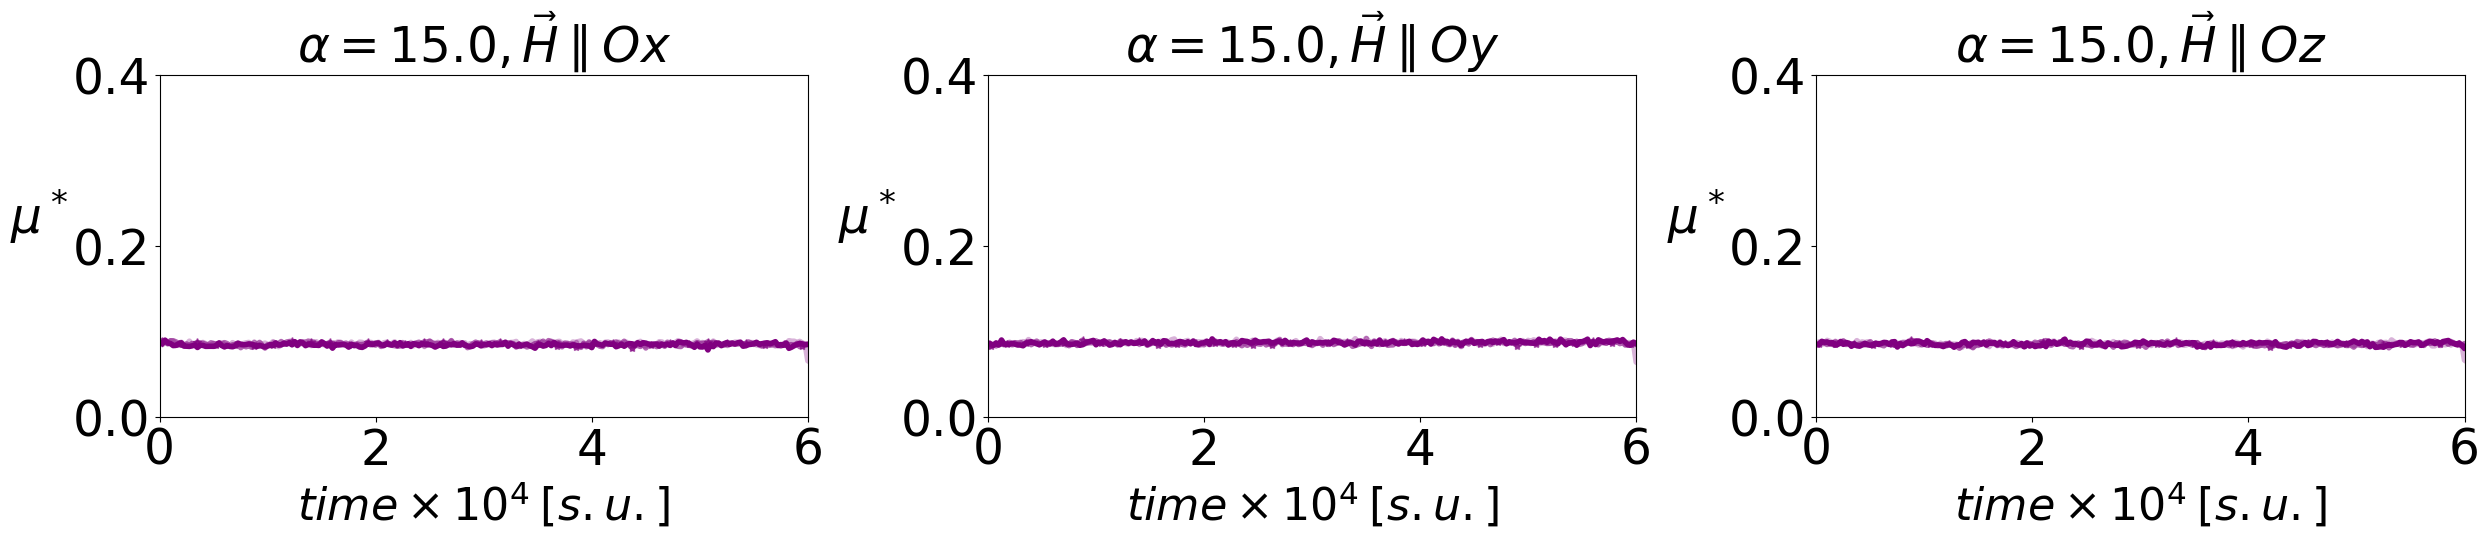} }
\end{minipage}
\vfill

\begin{minipage}[h]{\linewidth}
\center{\includegraphics[width=0.7\linewidth]{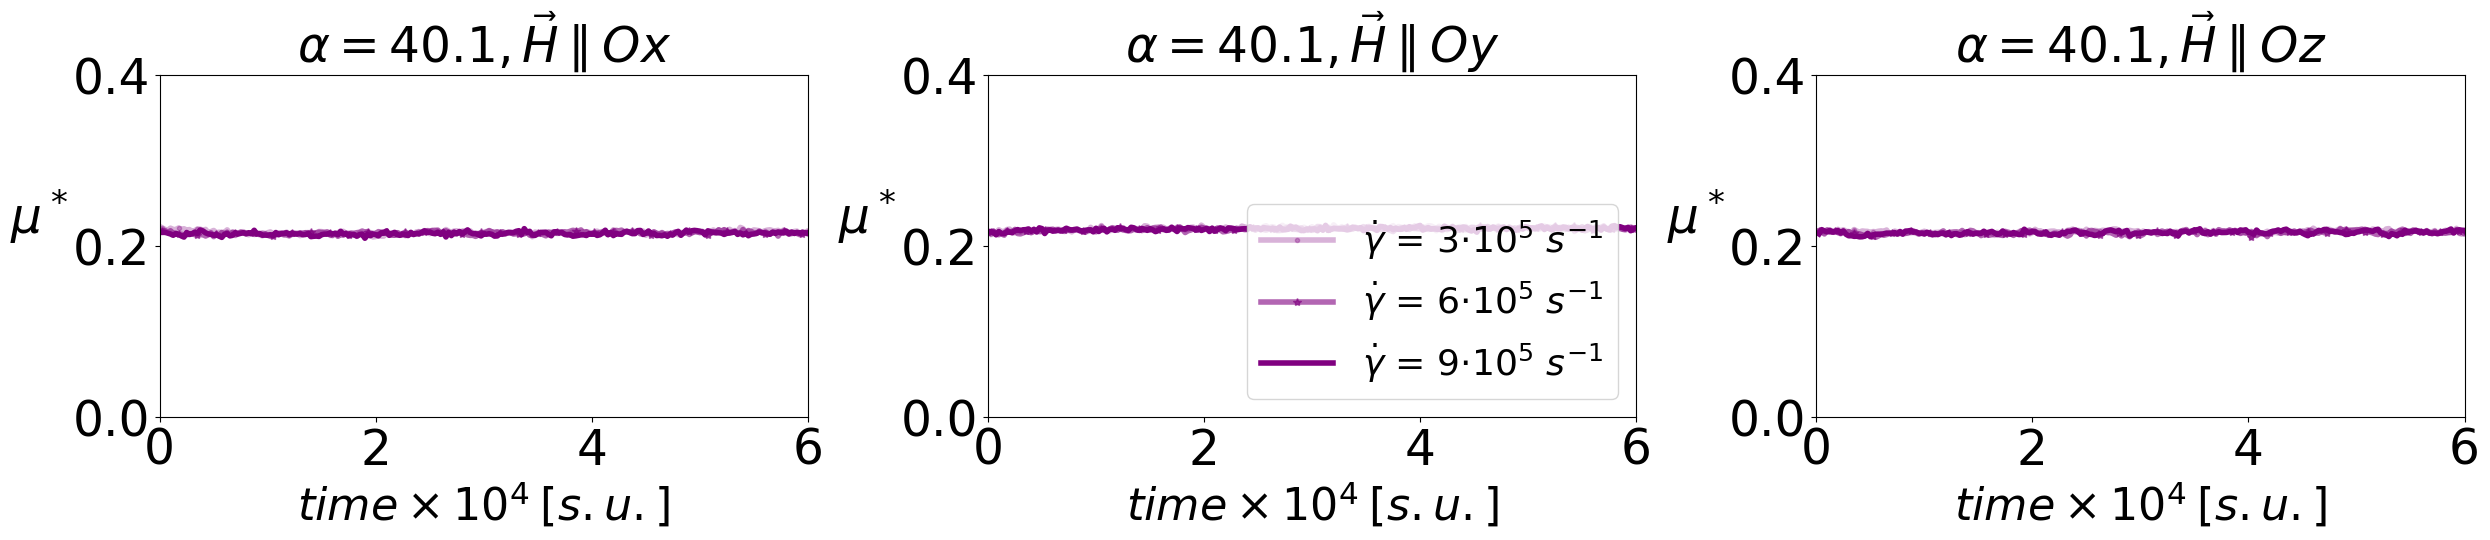} }
\end{minipage}
\caption{Dynamics of the magnetisation $\mu^{\ast}$ for a ring topology of the SSMPs. Columns correspond to a given orientation of the applied field. The brightness of the curves corresponds to the value of the shear rate -- the darker the curve, the higher the value of $\dot{\gamma}$. Exact $\dot{\gamma}$ values are provided in the inset of central figure. Field is fixed within each row. Values of $\alpha$ are provided above the plots.}
\end{figure*}

\begin{figure*}[h]
\begin{minipage}[h]{\linewidth}
\center{\includegraphics[width=0.7\linewidth]{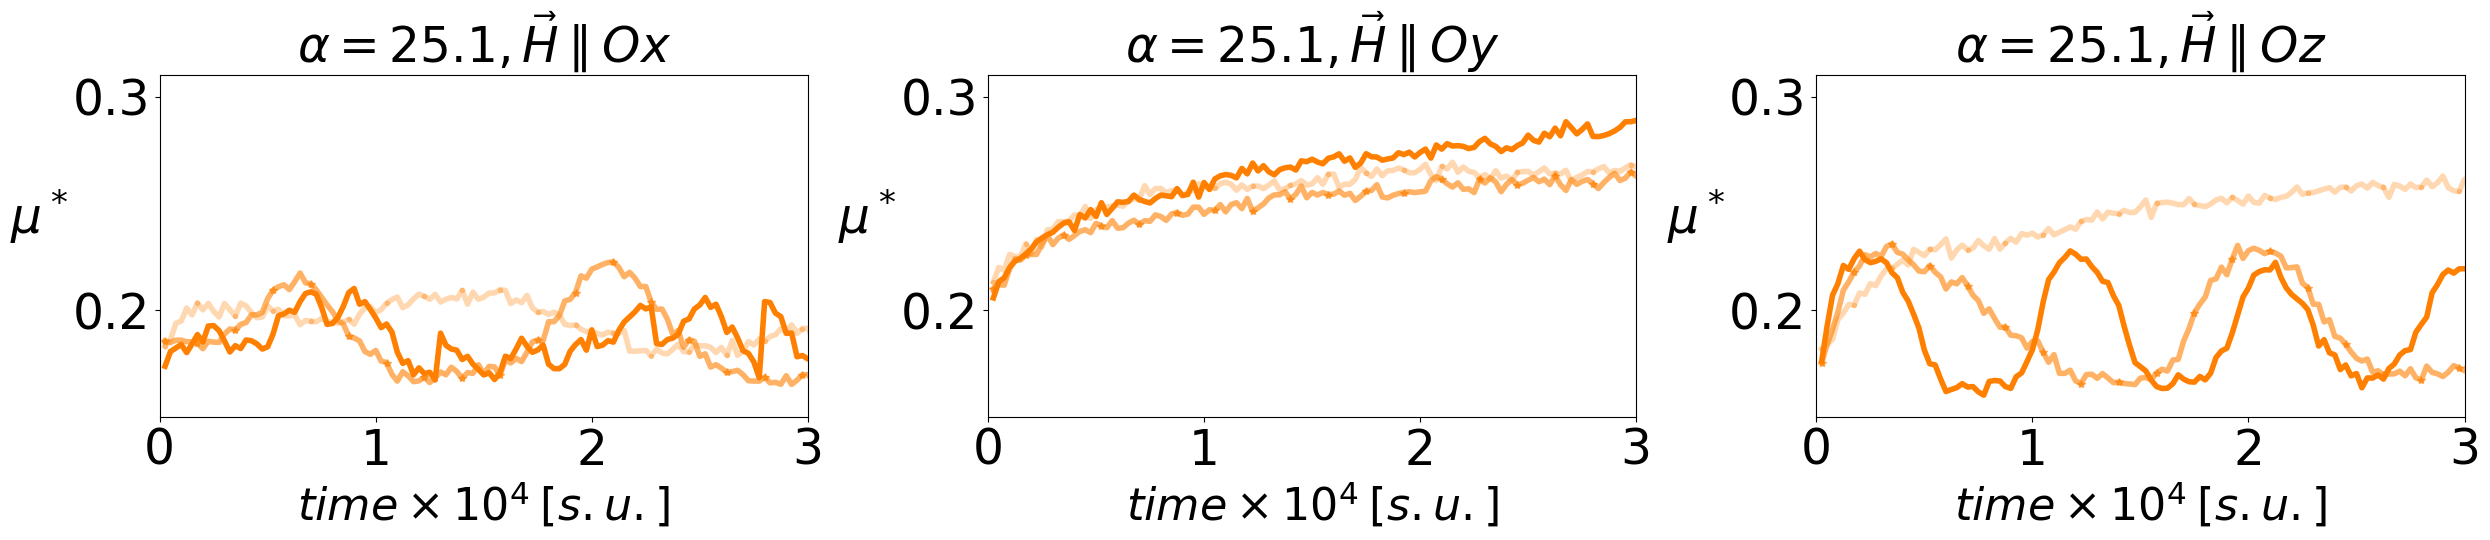} }
\end{minipage}
\vfill
\begin{minipage}[h]{\linewidth}
\center{\includegraphics[width=0.7\linewidth]{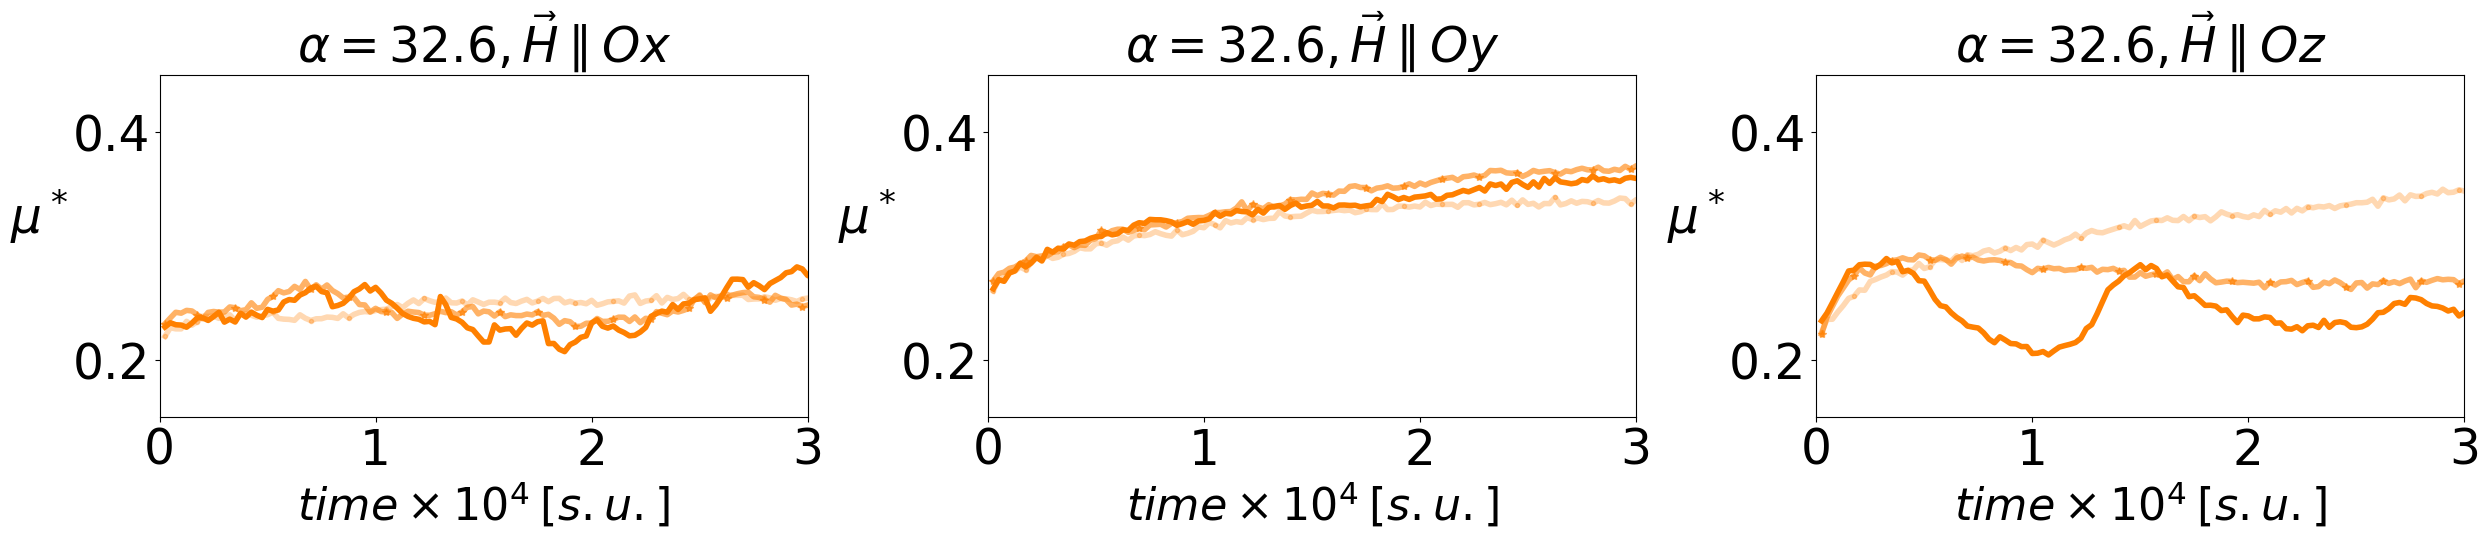} }
\end{minipage}
\vfill
\begin{minipage}[h]{\linewidth}
\center{\includegraphics[width=0.7\linewidth]{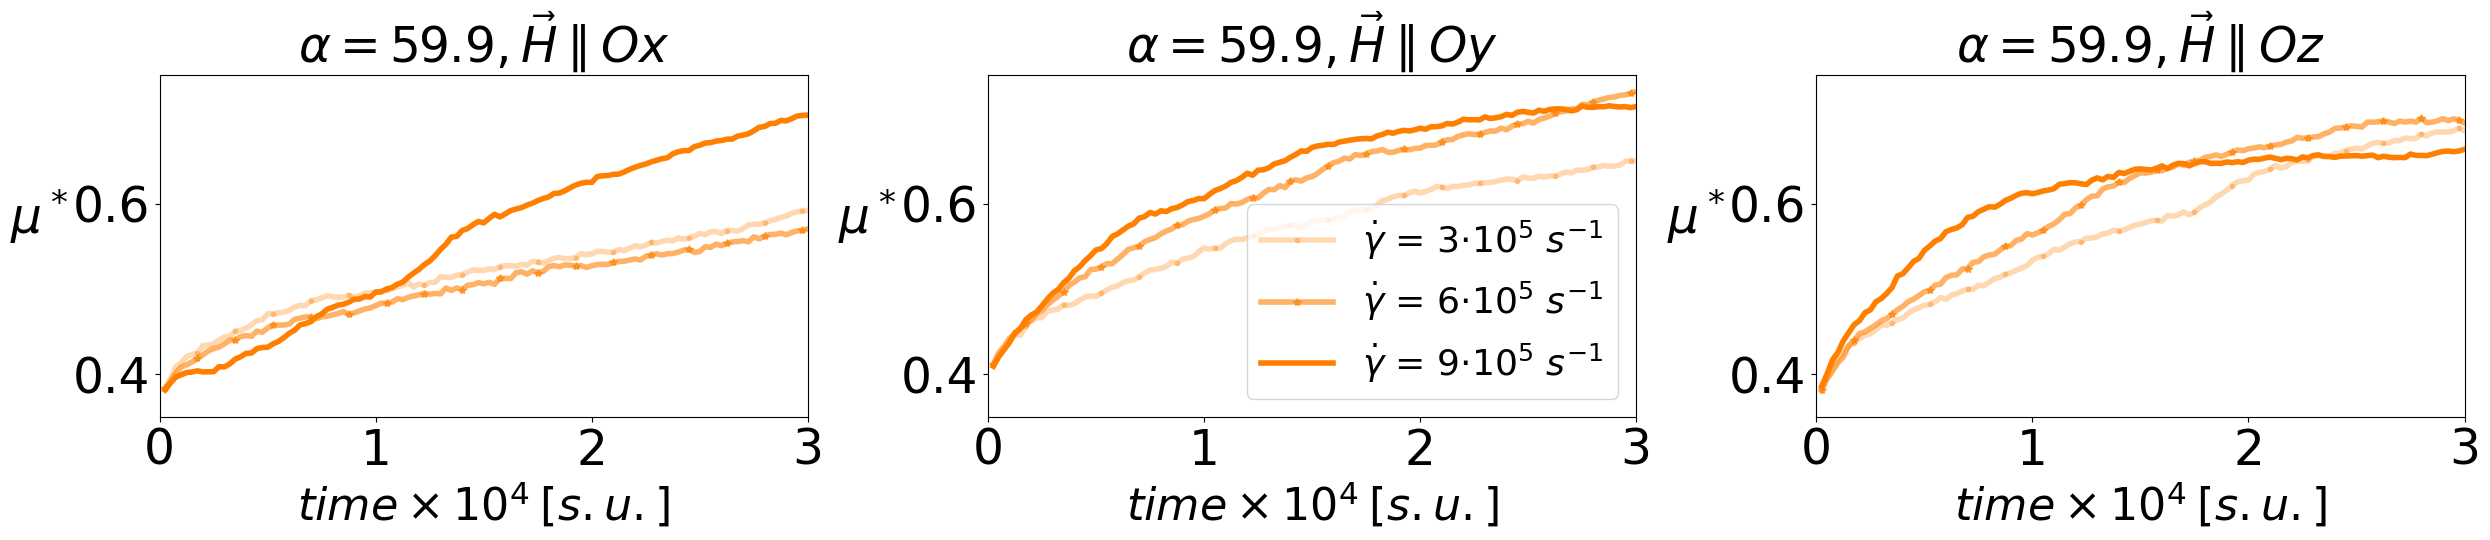} }
\end{minipage}
\caption{Dynamics of the magnetisation $\mu^{\ast}$ for a chain topology of the SSMPs. Columns correspond to a given orientation of the applied field. The brightness of the curves corresponds to the value of the shear rate -- the darker the curve, the higher the value of $\dot{\gamma}$. Exact $\dot{\gamma}$ values are provided in the inset of central. Field is fixed within each row. Values of $\alpha$ are provided above the plots.}
\end{figure*}

Additionally, we recommend the reader to watch supplementary videos. 

\end{document}
